# Supplementary material for: Adversarially Guided Stateful Defense Against Backdoor Attacks in Federated Deep Learning
Source: arXiv:2410.11205 source file (2024-10-15)

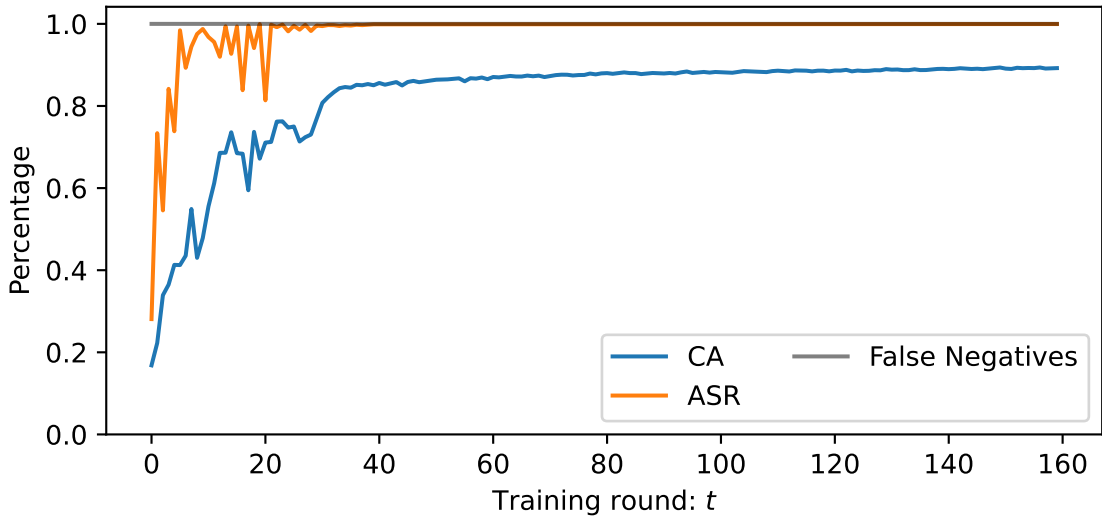

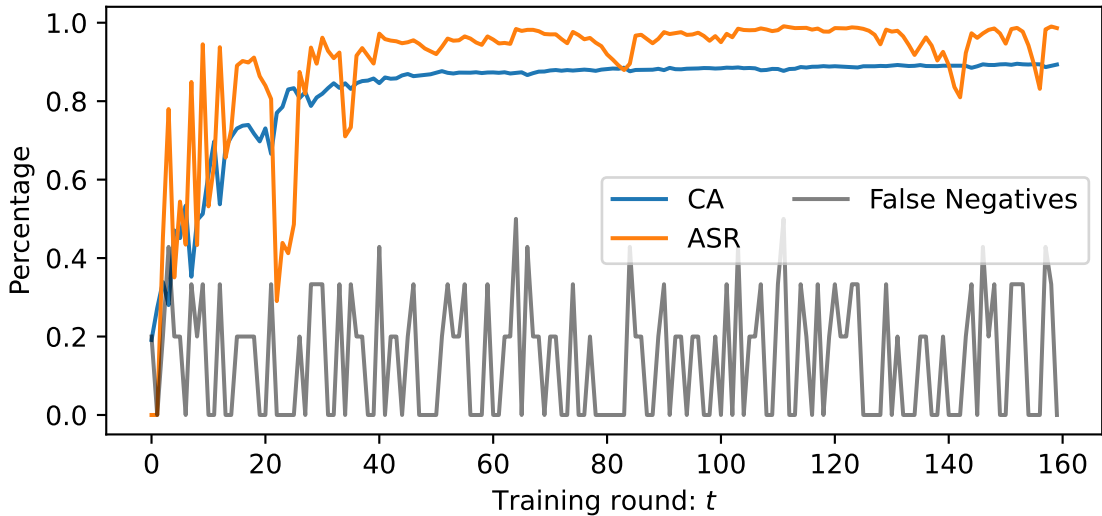

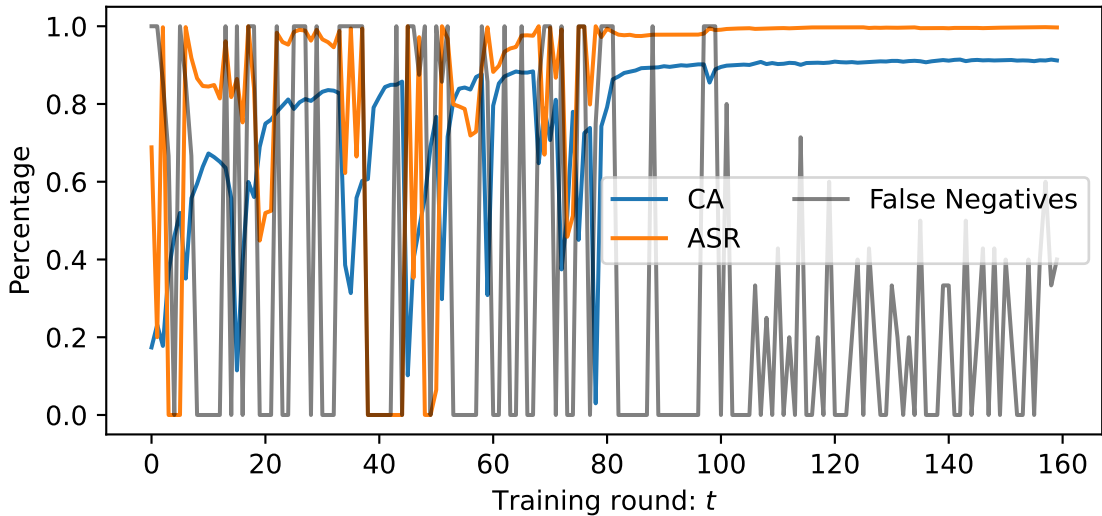

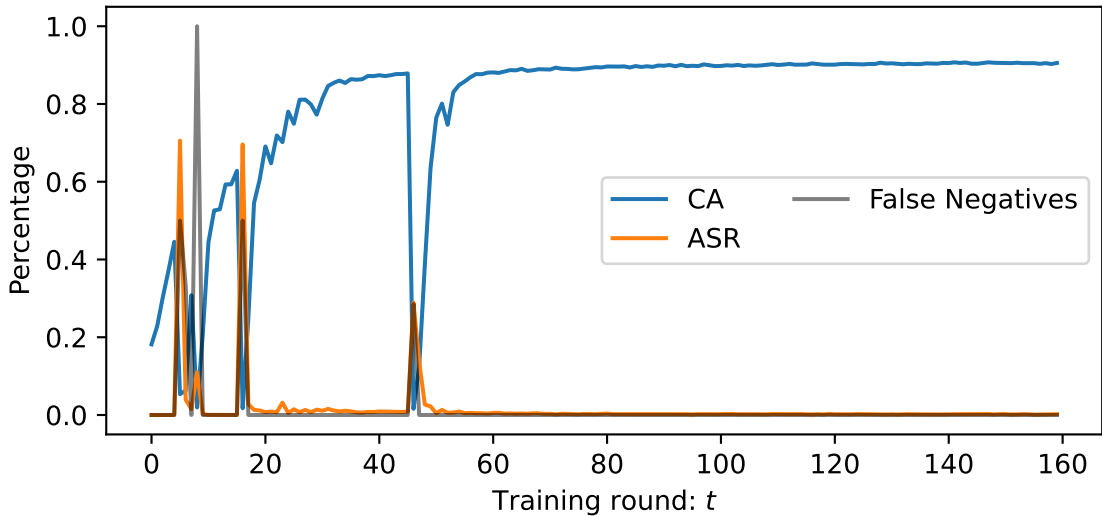

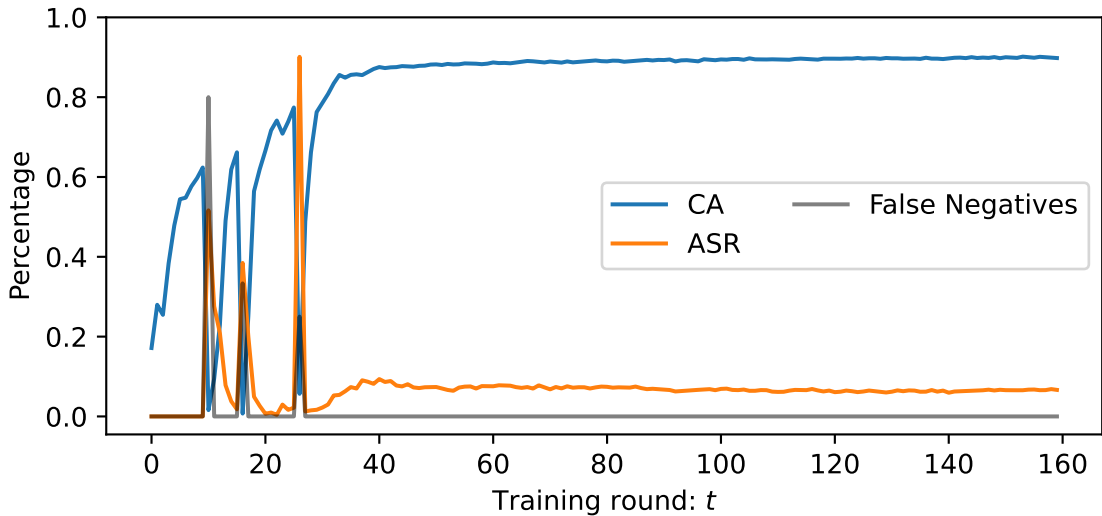

Supplement: Supplementary file 1 [file gtsrb_non_sota_adaptive_analysis_lba.pdf]
