# Supplementary material for: Adversarially Guided Stateful Defense Against Backdoor Attacks in Federated Deep Learning
Source: arXiv:2410.11205 source file (2024-10-15)

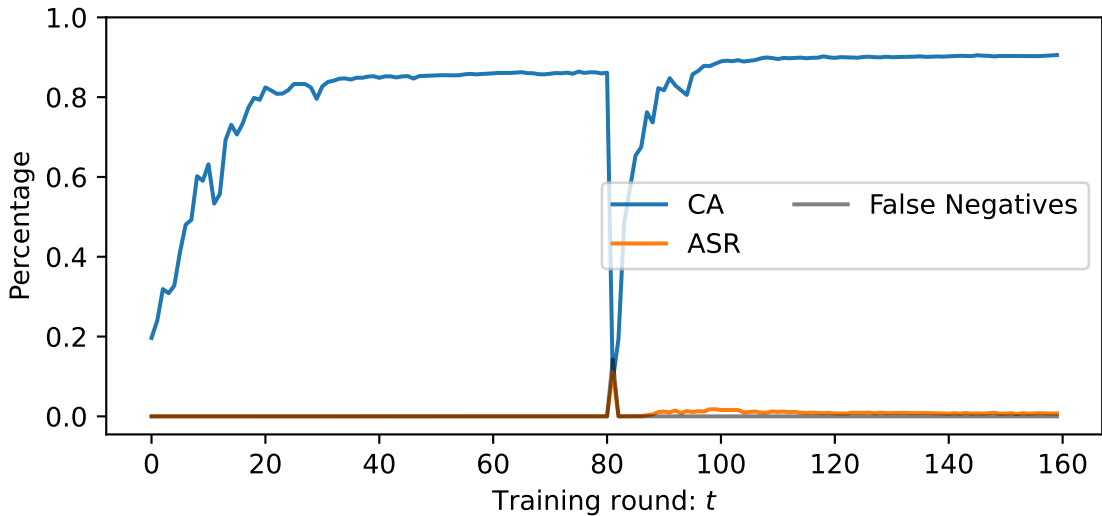

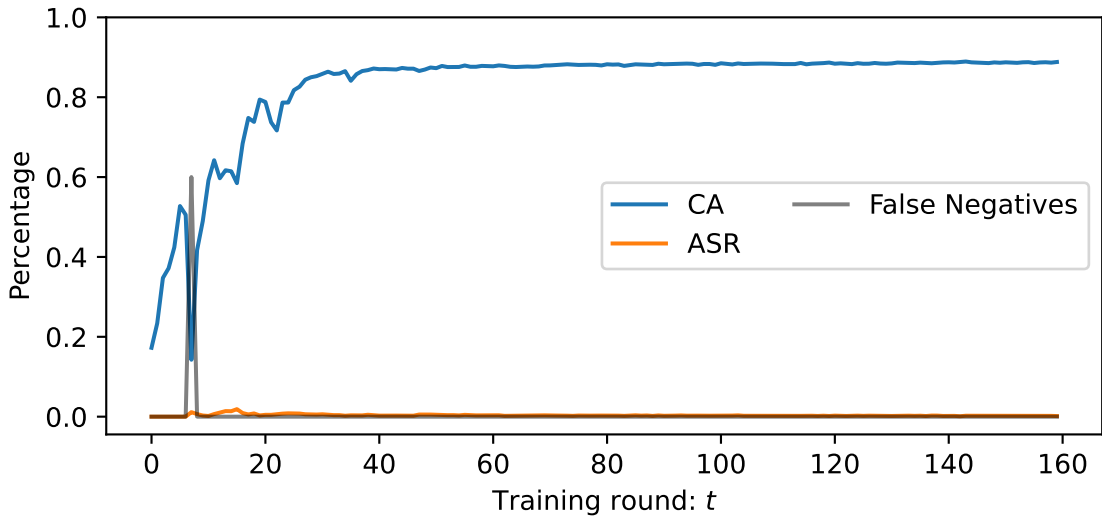

Supplement: Supplementary file 4 [file gtsrb_non_sota_malicious_clients_outnumber_clean_55.pdf]
