# Supplementary material for: Adversarially Guided Stateful Defense Against Backdoor Attacks in Federated Deep Learning
Source: arXiv:2410.11205 source file (2024-10-15)

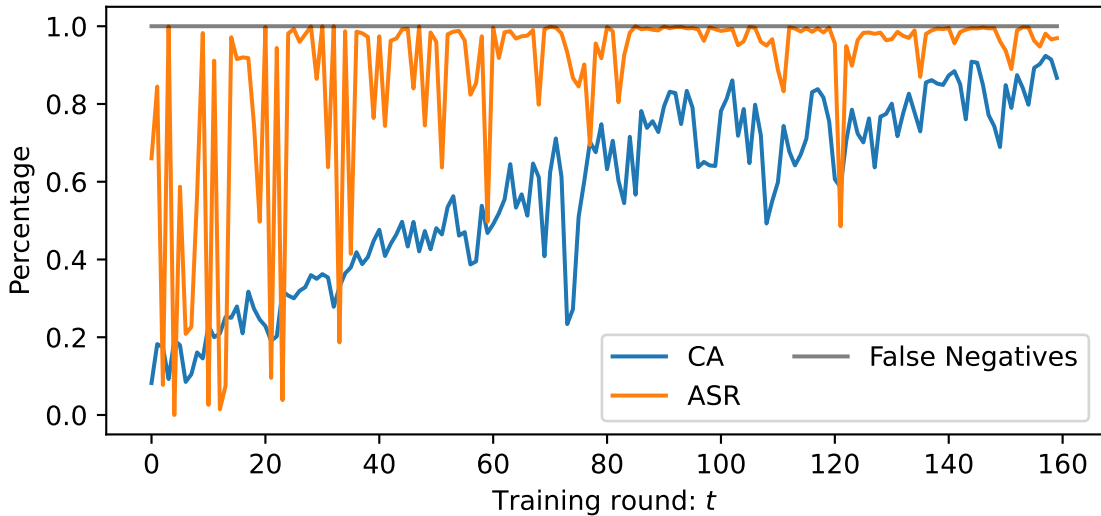

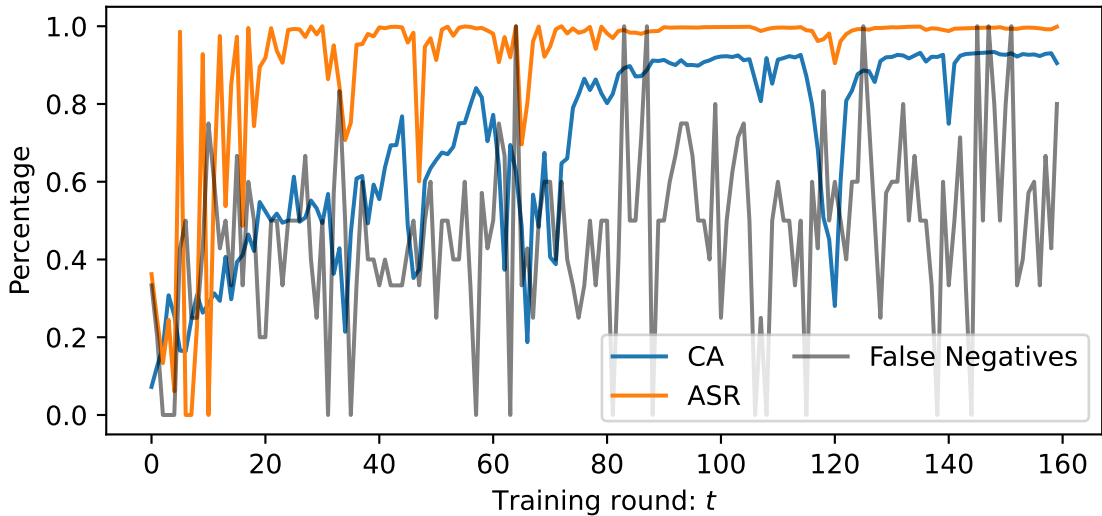

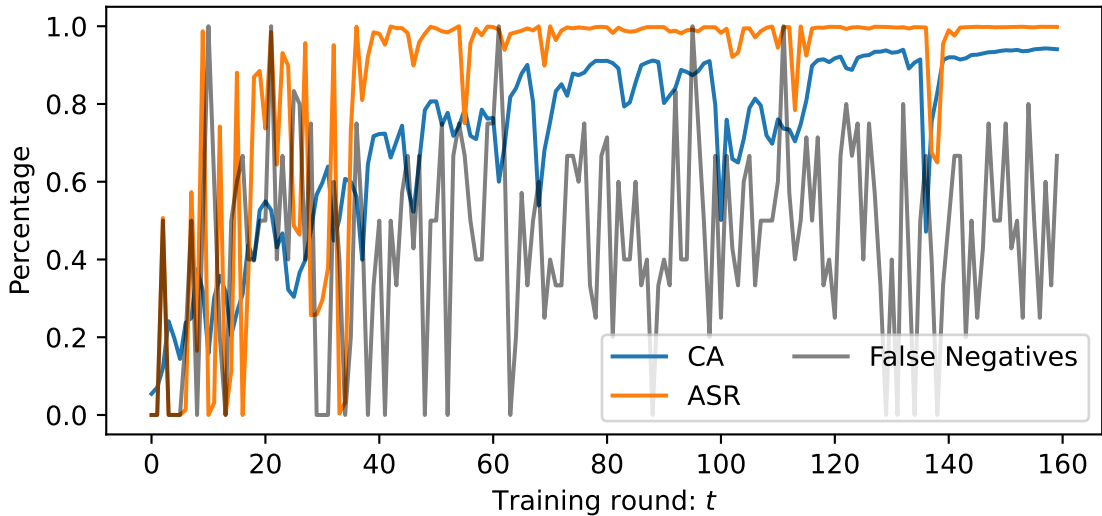

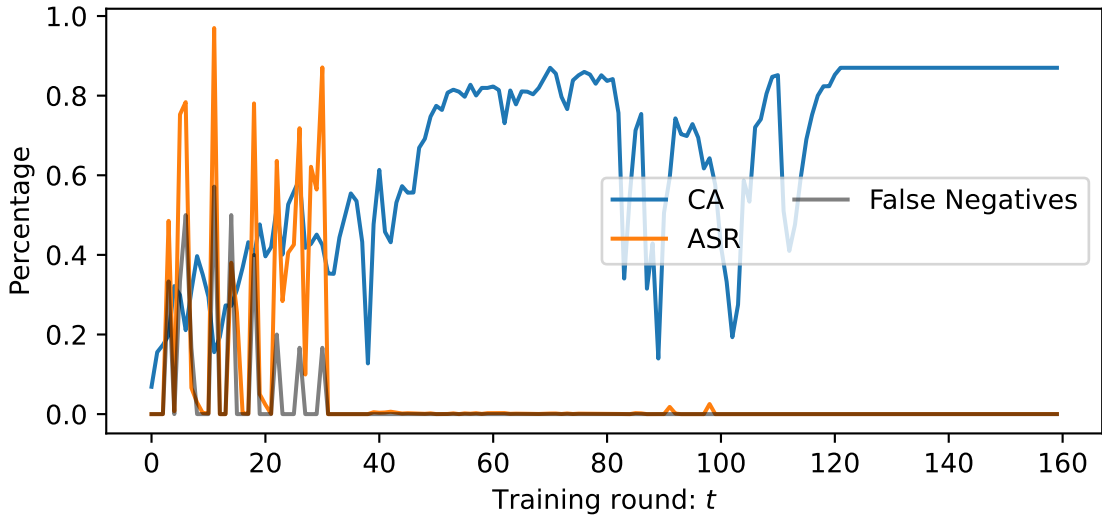

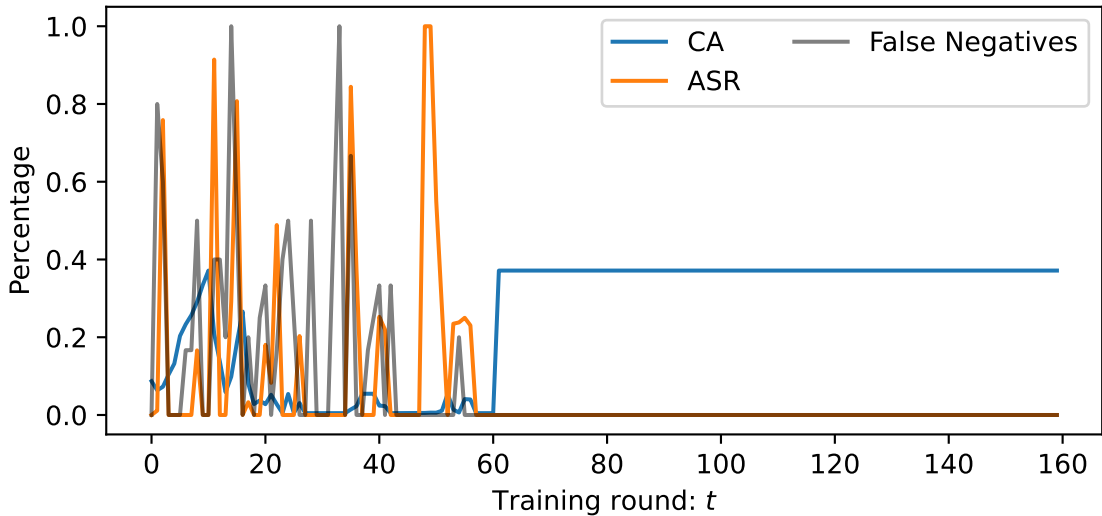

Supplement: Supplementary file 10 [file gtsrb_non_sota_standard_non_iid5_standard_noniid.pdf]
